# Supplementary material for: Differential cross section measurement of charged current $\nu_{e}$ interactions without final-state pions in MicroBooNE
Source: arXiv:2208.02348 ancillary file (2022-08-03)
Supplement: Supplementary file 1 [file Supplemental_Material.pdf]

# Differential cross section measurement of charged current $\nu_e$ interactions without final-state pions in MicroBooNE: Supplementary Material

P. Abratenko,<sup>34</sup> J. Anthony,<sup>4</sup> L. Arellano,<sup>19</sup> J. Asaadi,<sup>33</sup> A. Ashkenazi,<sup>31</sup> S. Balasubramanian,<sup>11</sup> B. Baller,<sup>11</sup> C. Barnes,<sup>21</sup> G. Barr,<sup>24</sup> J. Barrow,<sup>20,31</sup> V. Basque,<sup>11</sup> L. Bathe-Peters,<sup>13</sup> O. Benevides Rodrigues,<sup>30</sup> S. Berkman,<sup>11</sup> A. Bhandari,<sup>19</sup> M. Bhattacharya,<sup>11</sup> M. Bishai,<sup>2</sup> A. Blake,<sup>16</sup> B. Bogart,<sup>21</sup> T. Bolton,<sup>15</sup> J. Y. Book,<sup>13</sup> L. Camilleri,<sup>9</sup> D. Caratelli,<sup>3</sup> I. Caro Terrazas,<sup>8</sup> F. Cavanna,<sup>11</sup> G. Cerati,<sup>11</sup> Y. Chen,<sup>27</sup> J. M. Conrad,<sup>20</sup> M. Convery,<sup>27</sup> L. Cooper-Troendle,<sup>37</sup> J. I. Crespo-Anadón,<sup>5</sup> M. Del Tutto,<sup>11</sup> S. R. Dennis,<sup>4</sup> P. Detje,<sup>4</sup> A. Devitt,<sup>16</sup> R. Diurba,<sup>1,22</sup> R. Dorrill,<sup>14</sup> K. Duffy,<sup>24</sup> S. Dytman,<sup>25</sup> B. Eberly,<sup>29</sup> A. Ereditato,<sup>1</sup> J. J. Evans,<sup>19</sup> R. Fine,<sup>17</sup> O. G. Finnerud,<sup>19</sup> W. Foreman,<sup>14</sup> B. T. Fleming,<sup>37</sup> N. Foppiani,<sup>13</sup> D. Franco,<sup>37</sup> A. P. Furmanski,<sup>22</sup> D. Garcia-Gamez,<sup>12</sup> S. Gardiner,<sup>11</sup> G. Ge,<sup>9</sup> S. Gollapinni,<sup>32,17</sup> O. Goodwin,<sup>19</sup> E. Gramellini,<sup>11</sup> P. Green,<sup>19</sup> H. Greenlee,<sup>11</sup> W. Gu,<sup>2</sup> R. Guenette,<sup>19</sup> P. Guzowski,<sup>19</sup> L. Hagaman,<sup>37</sup> O. Hen,<sup>20</sup> R. Hicks,<sup>17</sup> C. Hilgenberg,<sup>22</sup> G. A. Horton-Smith,<sup>15</sup> B. Irwin,<sup>22</sup> R. Itay,<sup>27</sup> C. James,<sup>11</sup> X. Ji,<sup>2</sup> L. Jiang,<sup>35</sup> J. H. Jo,<sup>37</sup> R. A. Johnson,<sup>7</sup> Y.-J. Jwa,<sup>9</sup> D. Kalra,<sup>9</sup> N. Kamp,<sup>20</sup> G. Karagiorgi,<sup>9</sup> W. Ketchum,<sup>11</sup> M. Kirby,<sup>11</sup> T. Kobilarcik,<sup>11</sup> I. Kreslo,<sup>1</sup> M. B. Leibovitch,<sup>3</sup> I. Lepetic,<sup>26</sup> J.-Y. Li,<sup>10</sup> K. Li,<sup>37</sup> Y. Li,<sup>2</sup> K. Lin,<sup>26</sup> B. R. Littlejohn,<sup>14</sup> W. C. Louis,<sup>17</sup> X. Luo,<sup>3</sup> K. Manivannan,<sup>30</sup> C. Mariani,<sup>35</sup> D. Marsden,<sup>19</sup> J. Marshall,<sup>36</sup> D. A. Martinez Caicedo,<sup>28</sup> K. Mason,<sup>34</sup> A. Mastbaum,<sup>26</sup> N. McConkey,<sup>19</sup> V. Meddage,<sup>15</sup> K. Miller,<sup>6</sup> J. Mills,<sup>34</sup> A. Mogan,<sup>8</sup> T. Mohayai,<sup>11</sup> M. Mooney,<sup>8</sup> A. F. Moor,<sup>4</sup> C. D. Moore,<sup>11</sup> L. Mora Lepin,<sup>19</sup> J. Mousseau,<sup>21</sup> S. Mullerlababu,<sup>1</sup> D. Naples,<sup>25</sup> A. Navrer-Agasson,<sup>19</sup> N. Nayak,<sup>2</sup> M. Nebot-Guinot,<sup>10</sup> D. A. Newmark,<sup>17</sup> J. Nowak,<sup>16</sup> M. Nunes,<sup>30</sup> N. Oza,<sup>17</sup> O. Palamara,<sup>11</sup> N. Pallat,<sup>22</sup> V. Paolone,<sup>25</sup> A. Papadopoulou,<sup>20</sup> V. Papavassiliou,<sup>23</sup> H. B. Parkinson,<sup>10</sup> S. F. Pate,<sup>23</sup> N. Patel,<sup>16</sup> Z. Pavlovic,<sup>11</sup> E. Piasetzky,<sup>31</sup> I. D. Ponce-Pinto,<sup>37</sup> S. Prince,<sup>13</sup> X. Qian,<sup>2</sup> J. L. Raaf,<sup>11</sup> V. Radeka,<sup>2</sup> M. Reggiani-Guzzo,<sup>19</sup> L. Ren,<sup>23</sup> L. Rochester,<sup>27</sup> J. Rodriguez Rondon,<sup>28</sup> M. Rosenberg,<sup>34</sup> M. Ross-Lonergan,<sup>9,17</sup> C. Rudolf von Rohr,<sup>1</sup> G. Scanavini,<sup>37</sup> D. W. Schmitz,<sup>6</sup> A. Schukraft,<sup>11</sup> W. Seligman,<sup>9</sup> M. H. Shaevitz,<sup>9</sup> R. Sharankova,<sup>11</sup> J. Shi,<sup>4</sup> A. Smith,<sup>4</sup> E. L. Snider,<sup>11</sup> M. Soderberg,<sup>30</sup> S. Söldner-Rembold,<sup>19</sup> J. Spitz,<sup>21</sup> M. Stancari,<sup>11</sup> J. St. John,<sup>11</sup> T. Strauss,<sup>11</sup> S. Sword-Fehlberg,<sup>23</sup> A. M. Szec,<sup>10</sup> W. Tang,<sup>32</sup> N. Taniuchi,<sup>4</sup> K. Terao,<sup>27</sup> C. Thorpe,<sup>16</sup> D. Torbunov,<sup>2</sup> D. Totani,<sup>3</sup> M. Touns,<sup>11</sup> Y.-T. Tsai,<sup>27</sup> J. Tyler,<sup>15</sup> M. A. Uchida,<sup>4</sup> T. Usher,<sup>27</sup> B. Viren,<sup>2</sup> M. Weber,<sup>1</sup> H. Wei,<sup>18</sup> A. J. White,<sup>37</sup> Z. Williams,<sup>33</sup> S. Wolbers,<sup>11</sup> T. Wongjirad,<sup>34</sup> M. Wospakrik,<sup>11</sup> K. Wresilo,<sup>4</sup> N. Wright,<sup>20</sup> W. Wu,<sup>11</sup> E. Yandel,<sup>3</sup> T. Yang,<sup>11</sup> L. E. Yates,<sup>11</sup> H. W. Yu,<sup>2</sup> G. P. Zeller,<sup>11</sup> J. Zennaro,<sup>11</sup> and C. Zhang<sup>2</sup>

(The MicroBooNE Collaboration)\*

<sup>1</sup>Universität Bern, Bern CH-3012, Switzerland

<sup>2</sup>Brookhaven National Laboratory (BNL), Upton, NY, 11973, USA

<sup>3</sup>University of California, Santa Barbara, CA, 93106, USA

<sup>4</sup>University of Cambridge, Cambridge CB3 0HE, United Kingdom

<sup>5</sup>Centro de Investigaciones Energéticas, Medioambientales y Tecnológicas (CIEMAT), Madrid E-28040, Spain

<sup>6</sup>University of Chicago, Chicago, IL, 60637, USA

<sup>7</sup>University of Cincinnati, Cincinnati, OH, 45221, USA

<sup>8</sup>Colorado State University, Fort Collins, CO, 80523, USA

<sup>9</sup>Columbia University, New York, NY, 10027, USA

<sup>10</sup>University of Edinburgh, Edinburgh EH9 3FD, United Kingdom

<sup>11</sup>Fermi National Accelerator Laboratory (FNAL), Batavia, IL 60510, USA

<sup>12</sup>Universidad de Granada, Granada E-18071, Spain

<sup>13</sup>Harvard University, Cambridge, MA 02138, USA

<sup>14</sup>Illinois Institute of Technology (IIT), Chicago, IL 60616, USA

<sup>15</sup>Kansas State University (KSU), Manhattan, KS, 66506, USA

<sup>16</sup>Lancaster University, Lancaster LA1 4YW, United Kingdom

<sup>17</sup>Los Alamos National Laboratory (LANL), Los Alamos, NM, 87545, USA

<sup>18</sup>Louisiana State University, Baton Rouge, LA, 70803, USA

<sup>19</sup>The University of Manchester, Manchester M13 9PL, United Kingdom

<sup>20</sup>Massachusetts Institute of Technology (MIT), Cambridge, MA, 02139, USA

<sup>21</sup>University of Michigan, Ann Arbor, MI, 48109, USA

<sup>22</sup>University of Minnesota, Minneapolis, MN, 55455, USA

<sup>23</sup>New Mexico State University (NMSU), Las Cruces, NM, 88003, USA

<sup>24</sup>University of Oxford, Oxford OX1 3RH, United Kingdom

<sup>25</sup>University of Pittsburgh, Pittsburgh, PA, 15260, USA

<sup>26</sup>Rutgers University, Piscataway, NJ, 08854, USA

<sup>27</sup>SLAC National Accelerator Laboratory, Menlo Park, CA, 94025, USA

<sup>28</sup>South Dakota School of Mines and Technology (SDSMT), Rapid City, SD, 57701, USA

<sup>29</sup>University of Southern Maine, Portland, ME, 04104, USA

<sup>30</sup>*Syracuse University, Syracuse, NY, 13244, USA*

<sup>31</sup>*Tel Aviv University, Tel Aviv, Israel, 69978*

<sup>32</sup>*University of Tennessee, Knoxville, TN, 37996, USA*

<sup>33</sup>*University of Texas, Arlington, TX, 76019, USA*

<sup>34</sup>*Tufts University, Medford, MA, 02155, USA*

<sup>35</sup>*Center for Neutrino Physics, Virginia Tech, Blacksburg, VA, 24061, USA*

<sup>36</sup>*University of Warwick, Coventry CV4 7AL, United Kingdom*

<sup>37</sup>*Wright Laboratory, Department of Physics, Yale University, New Haven, CT, 06520, USA*

(Dated: August 3, 2022)

## I. PROTON THRESHOLD

The choice of the proton threshold at 50 MeV is motivated by Fig. 1, where we show the expected number of selected signal events as a function of the true leading proton kinetic energy for the  $1e0p0\pi$  and  $1eNp0\pi$  selections. The choice of 50 MeV corresponds to the energy where the two curves intersect, so below this value most events are selected with the  $1e0p0\pi$  selection, while above this value most events are selected with the  $1eNp0\pi$  selection.

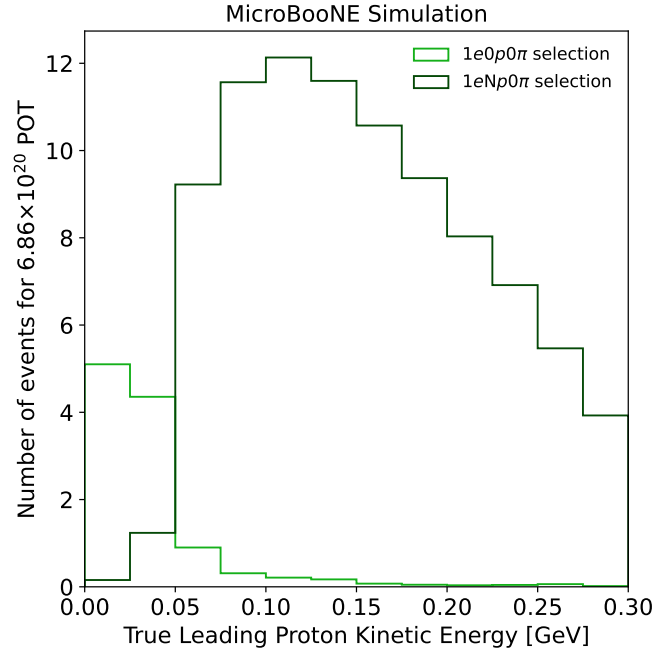

FIG. 1. Expected number of signal events for  $6.86 \times 10^{20}$  POT as a function of the leading proton kinetic energy for the  $1e0p0\pi$  and  $1eNp0\pi$  selections.

---

\* microboone.info@fnal.gov

## II. INTERACTION MODE OF SELECTED EVENTS

In addition to true visible final state the selected neutrino events can also be classified by true interaction mode. The interaction mode breakdown for the tuned version of GENIE v3 is shown in Fig. 2 for events passing the cross-section selection in all four variables in which the cross section is measured.

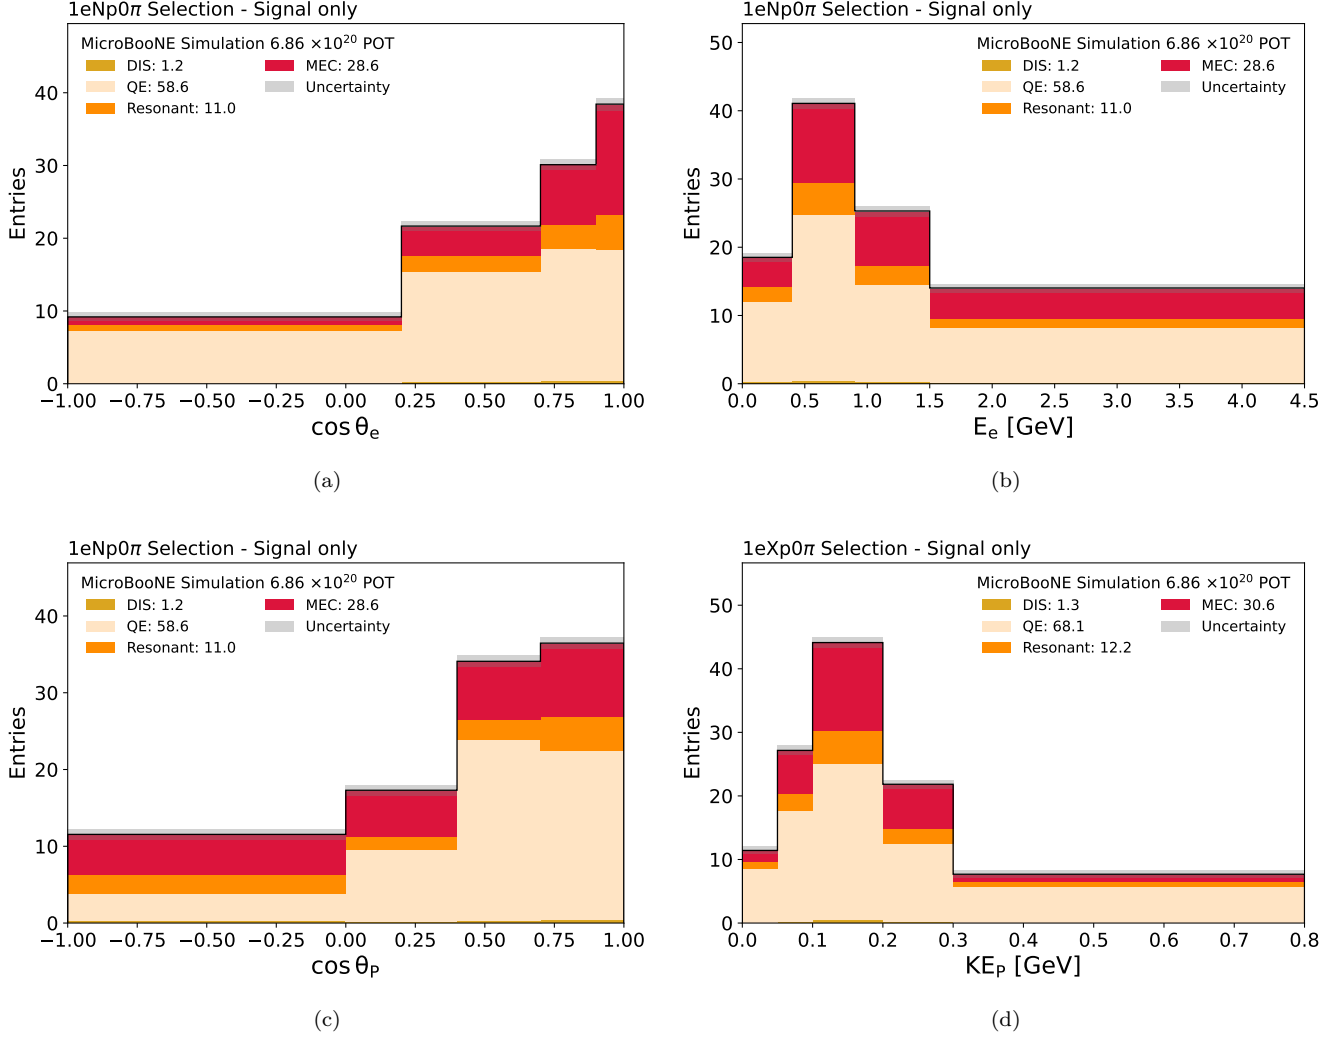

FIG. 2. Signal prediction using the MicroBooNE tune of GENIE v3 after selection, categorized by interaction mode: quasi-elastic (QE), meson exchange current (MEC), resonant, and deep inelastic scattering (DIS). The prediction is shown in (a) the angle between the neutrino beam and the electron direction, (b) electron kinetic energy, (c) the angle between the neutrino beam and the leading proton direction, and (d) the leading proton kinetic energy. The uncertainty band includes only statistical uncertainties of the simulated samples.

### III. ELECTRON ENERGY

The tables in this section provide additional information for the cross-section measurement as a function of the electron energy: background-subtracted observation and cross-section values (Table I),  $\chi^2$  values for the different generators tests (Table II), covariance matrices for the extracted cross section (Table III) and for the background-subtracted data prediction (Table IV), and response matrix (Table V).

TABLE I. Unfolded cross section as a function of electron energy.

| Bin [GeV]                                                | [0, 0.4] | [0.4, 0.9] | [0.9, 1.5] | [1.5, 4.5] |
|----------------------------------------------------------|----------|------------|------------|------------|
| Background-subtracted data events                        | 11.86    | 21.75      | 15.11      | 14.80      |
| Cross section [ $10^{-39}$ cm <sup>2</sup> /GeV/nucleon] | 1.86     | 1.76       | 0.99       | 0.31       |

TABLE II. Results of compatibility tests between generators and the measured cross-section as a function of electron energy.

|            | GENIE v3 uB | GENIE v3 | GENIE v2 | NuWro | NEUT  |
|------------|-------------|----------|----------|-------|-------|
| $\chi^2$   | 6.83        | 2.75     | 6.39     | 4.30  | 9.12  |
| d.o.f.     | 4           | 4        | 4        | 4     | 4     |
| $p$ -value | 0.145       | 0.600    | 0.172    | 0.367 | 0.058 |

TABLE III. Covariance matrix for the cross section measurement as a function of electron energy. Units are (cm<sup>2</sup>/GeV/nucleon)<sup>2</sup>.

| Bin [GeV]  | [0, 0.4]  | [0.4, 0.9] | [0.9, 1.5] | [1.5, 4.5] |
|------------|-----------|------------|------------|------------|
| [0, 0.4]   | 2.46e-78  | 1.07e-79   | -5.40e-81  | 8.67e-81   |
| [0.4, 0.9] | 1.07e-79  | 6.68e-79   | 2.04e-80   | 5.96e-82   |
| [0.9, 1.5] | -5.40e-81 | 2.04e-80   | 2.60e-79   | 4.24e-82   |
| [1.5, 4.5] | 8.67e-81  | 5.96e-82   | 4.24e-82   | 1.21e-80   |

TABLE IV. Covariance matrix for the total event prediction as a function of electron energy.

| Bin [GeV]  | [0, 0.4] | [0.4, 0.9] | [0.9, 1.5] | [1.5, 4.5] |
|------------|----------|------------|------------|------------|
| [0, 0.4]   | 63.99    | 13.57      | 4.59       | 2.44       |
| [0.4, 0.9] | 13.57    | 76.73      | 7.32       | 4.17       |
| [0.9, 1.5] | 4.59     | 7.32       | 44.73      | 3.07       |
| [1.5, 4.5] | 2.44     | 4.17       | 3.07       | 29.27      |

TABLE V. Response matrix for signal events as a function of electron energy.

| Bin [GeV]  | [0, 0.4] | [0.4, 0.9] | [0.9, 1.5] | [1.5, 4.5] |
|------------|----------|------------|------------|------------|
| [0, 0.4]   | 0.097    | 0.026      | 0.003      | 0.001      |
| [0.4, 0.9] | 0.012    | 0.156      | 0.053      | 0.005      |
| [0.9, 1.5] | 0.000    | 0.010      | 0.144      | 0.040      |
| [1.5, 4.5] | 0.000    | 0.000      | 0.007      | 0.126      |

#### IV. ELECTRON ANGLE

The tables in this section provide additional information for the cross-section measurement as a function of the electron angle: background-subtracted observation and cross-section values (Table VI),  $\chi^2$  values for the different generators tests (Table VII), covariance matrices for the extracted cross section (Table VIII) and for the background-subtracted data prediction (Table IX), and response matrix (Table X).

TABLE VI. Unfolded cross section as a function of electron angle.

| Bin                                                  | $[-1, 0.2]$ | $[0.2, 0.7]$ | $[0.7, 0.9]$ | $[0.9, 1]$ |
|------------------------------------------------------|-------------|--------------|--------------|------------|
| Background-subtracted data events                    | 5.96        | 13.73        | 17.98        | 27.20      |
| Cross section [ $10^{-39}$ cm <sup>2</sup> /nucleon] | 0.47        | 1.41         | 3.71         | 10.94      |

TABLE VII. Results of compatibility tests between generators and the measured cross-section as a function of electron angle.

|            | GENIE v3 uB | GENIE v3 | GENIE v2 | NuWro | NEUT  |
|------------|-------------|----------|----------|-------|-------|
| $\chi^2$   | 4.67        | 0.95     | 4.70     | 2.14  | 6.56  |
| d.o.f.     | 4           | 4        | 4        | 4     | 4     |
| $p$ -value | 0.322       | 0.917    | 0.319    | 0.710 | 0.161 |

TABLE VIII. Covariance matrix for the cross section measurement as a function of electron angle. Units are (cm<sup>2</sup>/nucleon)<sup>2</sup>.

| Bin          | $[-1, 0.2]$ | $[0.2, 0.7]$ | $[0.7, 0.9]$ | $[0.9, 1]$ |
|--------------|-------------|--------------|--------------|------------|
| $[-1, 0.2]$  | 1.99e-79    | 2.07e-80     | 8.05e-80     | 1.14e-79   |
| $[0.2, 0.7]$ | 2.07e-80    | 4.81e-79     | 9.68e-80     | 2.29e-79   |
| $[0.7, 0.9]$ | 8.05e-80    | 9.68e-80     | 2.82e-78     | 3.86e-79   |
| $[0.9, 1]$   | 1.14e-79    | 2.29e-79     | 3.86e-79     | 1.26e-77   |

TABLE IX. Covariance matrix for the total event prediction as a function of electron angle.

| Bin          | $[-1, 0.2]$ | $[0.2, 0.7]$ | $[0.7, 0.9]$ | $[0.9, 1]$ |
|--------------|-------------|--------------|--------------|------------|
| $[-1, 0.2]$  | 29.30       | 4.24         | 4.74         | 3.63       |
| $[0.2, 0.7]$ | 4.24        | 41.05        | 8.05         | 5.83       |
| $[0.7, 0.9]$ | 4.74        | 8.05         | 55.58        | 9.60       |
| $[0.9, 1]$   | 3.63        | 5.83         | 9.60         | 73.74      |

TABLE X. Response matrix for signal events as a function of electron angle.

| Bin          | $[-1, 0.2]$ | $[0.2, 0.7]$ | $[0.7, 0.9]$ | $[0.9, 1]$ |
|--------------|-------------|--------------|--------------|------------|
| $[-1, 0.2]$  | 0.084       | 0.003        | 0.000        | 0.000      |
| $[0.2, 0.7]$ | 0.003       | 0.152        | 0.007        | 0.000      |
| $[0.7, 0.9]$ | 0.000       | 0.009        | 0.182        | 0.008      |
| $[0.9, 1]$   | 0.000       | 0.000        | 0.010        | 0.201      |

## V. PROTON ENERGY

The tables in this section provide additional information for the cross-section measurement as a function of the proton kinetic energy: background-subtracted observation and cross-section values (Table [XI](#)),  $\chi^2$  values for the different generators tests (Table [XII](#)), covariance matrices for the extracted cross section (Table [XIII](#)) and for the background-subtracted data prediction (Table [XIV](#)), and response matrix (Table [XV](#)).

TABLE XI. Unfolded cross section as a function of proton energy.

| Bin [GeV]                                                | [0, 0.05] | [0.05, 0.1] | [0.1, 0.2] | [0.2, 0.3] | [0.3, 0.8] |
|----------------------------------------------------------|-----------|-------------|------------|------------|------------|
| Background-subtracted data events                        | 7.81      | 13.20       | 35.03      | 10.72      | 7.30       |
| Cross section [ $10^{-39}$ cm <sup>2</sup> /GeV/nucleon] | 10.15     | 9.32        | 13.66      | 4.49       | 1.72       |

TABLE XII. Results of compatibility tests between generators and the measured cross-section as a function of proton energy.

|            | GENIE v3 uB | GENIE v3 | GENIE v2 | NuWro | NEUT  |
|------------|-------------|----------|----------|-------|-------|
| $\chi^2$   | 6.35        | 2.41     | 7.53     | 2.73  | 6.85  |
| d.o.f.     | 4           | 4        | 4        | 4     | 4     |
| $p$ -value | 0.273       | 0.791    | 0.184    | 0.742 | 0.232 |

TABLE XIII. Covariance matrix for the cross section measurement as a function of proton energy. Units are (cm<sup>2</sup>/GeV/nucleon)<sup>2</sup>.

| Bin [GeV]   | [0, 0.05] | [0.05, 0.1] | [0.1, 0.2] | [0.2, 0.3] | [0.3, 0.8] |
|-------------|-----------|-------------|------------|------------|------------|
| [0, 0.05]   | 5.64e-77  | 1.06e-78    | 1.95e-78   | 1.16e-78   | 1.79e-79   |
| [0.05, 0.1] | 1.06e-78  | 5.82e-77    | 2.95e-78   | 1.65e-78   | 2.55e-79   |
| [0.1, 0.2]  | 1.95e-78  | 2.95e-78    | 1.46e-77   | 1.63e-79   | 5.19e-80   |
| [0.2, 0.3]  | 1.16e-78  | 1.65e-78    | 1.63e-79   | 8.33e-78   | 9.57e-80   |
| [0.3, 0.8]  | 1.70e-79  | 2.55e-79    | 5.19e-80   | 9.57e-80   | 7.11e-79   |

TABLE XIV. Covariance matrix for the total event prediction as a function of proton energy.

| Bin [GeV]   | [0, 0.05] | [0.05, 0.1] | [0.1, 0.2] | [0.2, 0.3] | [0.3, 0.8] |
|-------------|-----------|-------------|------------|------------|------------|
| [0, 0.05]   | 25.79     | 4.83        | 5.87       | 2.28       | 0.68       |
| [0.05, 0.1] | 4.83      | 60.84       | 13.28      | 5.46       | 1.52       |
| [0.1, 0.2]  | 5.87      | 13.28       | 85.58      | 7.69       | 2.20       |
| [0.2, 0.3]  | 2.28      | 5.46        | 7.69       | 37.20      | 2.08       |
| [0.3, 0.8]  | 0.68      | 1.52        | 2.20       | 2.08       | 13.31      |

TABLE XV. Response matrix for signal events as a function of proton energy.

| Bin [GeV]   | [0, 0.05] | [0.05, 0.1] | [0.1, 0.2] | [0.2, 0.3] | [0.3, 0.8] |
|-------------|-----------|-------------|------------|------------|------------|
| [0, 0.05]   | 0.108     | 0.009       | 0.003      | 0.001      | 0.001      |
| [0.05, 0.1] | 0.015     | 0.150       | 0.024      | 0.008      | 0.002      |
| [0.1, 0.2]  | 0.001     | 0.006       | 0.192      | 0.036      | 0.006      |
| [0.2, 0.3]  | 0.000     | 0.000       | 0.003      | 0.163      | 0.018      |
| [0.3, 0.8]  | 0.000     | 0.000       | 0.000      | 0.001      | 0.068      |

## VI. PROTON ANGLE

The tables in this section provide additional information for the cross-section measurement as a function of the proton angle: background-subtracted observation and cross-section values (Table XVI),  $\chi^2$  values for the different generators tests (Table XVII), covariance matrices for the extracted cross section (Table XVIII) and for the background-subtracted data prediction (Table XIX), and response matrix (Table XX).

TABLE XVI. Unfolded cross section as a function of proton angle.

| Bin                                                  | $[-1, 0]$ | $[0, 0.4]$ | $[0.4, 0.7]$ | $[0.7, 1]$ |
|------------------------------------------------------|-----------|------------|--------------|------------|
| Background subtracted data events                    | 7.09      | 23.80      | 16.74        | 17.22      |
| Cross section [ $10^{-39}$ cm <sup>2</sup> /nucleon] | 0.26      | 2.88       | 2.14         | 3.25       |

TABLE XVII. Results of compatibility tests between generators and the measured cross-section as a function of proton angle.

|            | GENIE v3 uB | GENIE v3 | GENIE v2 | NuWro | NEUT  |
|------------|-------------|----------|----------|-------|-------|
| $\chi^2$   | 11.86       | 8.63     | 12.64    | 9.98  | 14.55 |
| d.o.f.     | 4           | 4        | 4        | 4     | 4     |
| $p$ -value | 0.018       | 0.071    | 0.013    | 0.041 | 0.006 |

TABLE XVIII. Covariance matrix for the cross section measurement as a function of proton angle. Units are (cm<sup>2</sup>/nucleon)<sup>2</sup>.

| Bin          | $[-1, 0]$ | $[0, 0.4]$ | $[0.4, 0.7]$ | $[0.7, 1]$ |
|--------------|-----------|------------|--------------|------------|
| $[-1, 0]$    | 7.69e-80  | 1.02e-80   | 1.11e-80     | 5.50e-80   |
| $[0, 0.4]$   | 1.02e-80  | 4.51e-79   | -1.89e-80    | 6.47e-80   |
| $[0.4, 0.7]$ | 1.11e-80  | -1.89e-80  | 1.15e-78     | 1.25e-79   |
| $[0.7, 1]$   | 5.50e-80  | 6.47e-80   | 1.25e-79     | 3.88e-78   |

TABLE XIX. Covariance matrix for the total event prediction as a function of proton angle.

| Bin          | $[-1, 0]$ | $[0, 0.4]$ | $[0.4, 0.7]$ | $[0.7, 1]$ |
|--------------|-----------|------------|--------------|------------|
| $[-1, 0]$    | 29.52     | 3.02       | 3.80         | 8.21       |
| $[0, 0.4]$   | 3.02      | 28.10      | 3.93         | 6.81       |
| $[0.4, 0.7]$ | 3.80      | 3.93       | 52.33        | 10.99      |
| $[0.7, 1]$   | 8.21      | 6.81       | 10.99        | 86.76      |

TABLE XX. Response matrix for signal events as a function of proton angle.

| Bin          | $[-1, 0]$ | $[0, 0.4]$ | $[0.4, 0.7]$ | $[0.7, 1]$ |
|--------------|-----------|------------|--------------|------------|
| $[-1, 0]$    | 0.140     | 0.016      | 0.005        | 0.005      |
| $[0, 0.4]$   | 0.011     | 0.152      | 0.014        | 0.003      |
| $[0.4, 0.7]$ | 0.006     | 0.019      | 0.175        | 0.010      |
| $[0.7, 1]$   | 0.009     | 0.005      | 0.017        | 0.126      |
